# Supplementary material for: A stochastic approximation algorithm for stochastic semidefinite programming
Source: arXiv:1507.01859 source file (2015-07-07)
Supplement: Supplementary file 1 [file Appendix.tex]

\section{Unbiased estimators for $\bW^{-1}$ and $\bV_{k}$}
\label{app.estimation}

In this appendix, we present an unbiased procedure with which the receiver and the transmitters may estimate the physical quantities involved in the the discretization \eqref{eq.XLT.discrete} of \eqref{eq.XLT}, based at each step on direct signal measurements that may be subject to observational (but not systematic) errors.
%However this will not be detailled down to practical implementations because we do not feel that this is the main object of this paper. \bruno{Keep this sentence?}\mpierre{I would remove it}

We first consider the random perturbations induced on the measurement of $\bW$ by signal sampling at the receiver end.
To wit, recall that $\bW$ is just the covariance matrix of the aggregate received signal $\by\in\C^{m_{0}}$:
indeed,
%the signal model \eqref{eq.signal} yields
\(
%\begin{multline}
\ex[\by \by^{\dag}]
%	=\txs \ex \big[(\bz + \insum_{k} \bH_{k} \bx_{k}) \cdot (\bz + \insum_{\ell} \bH_{\ell} \bx_{\ell})^{\dag}\big]
%	\\
%	\notag\\
	=\txs \ex \big[\bz \bz^{\dag} \big] + \insum_{k} \bH_{k} \ex\big[\bx_{k} \bx_{k}^{\dag} \big] \bH_{k}^{\dag}
%	\notag\\
	=\txs \bI + \insum_{k} \bH_{k} \bQ_{k} \bH_{k}^{\dag}
	= \bW,
%\end{multline}
\)
so $\bP \eqdef \bW^{-1}$ is simply the precision (inverse covariance) matrix of a multivariate Gaussian random variable.

An unbiased estimate for the covariance $\bW$ of $\by$
%of the Gaussian random vector $\by$
may be obtained from a systematically unbiased sample $\by_{1},\dotsc, \by_{M}$ of $\by$ by means of the classical estimator $\hat \bW = \frac{1}{M} \insum_{j=1}^{M} \by_{j} \by_{j}^{\dag}$.%
\footnote{Since the expected value $\ex[\by] = 0$ of $\by$ need not be estimated itself from the data sample, we do not need to include the $M/(M-1)$ bias correction factor in the estimate of $\bW$.}
On the other hand, given that $\hat\bW^{-1}$ is a biased estimator of $\bW^{-1}$ (and hence introduces a systematic error to the measurement process) \cite{Anderson}, we cannot use this classical covariance estimate for $\bW^{-1}$.
Instead, following \cite{Anderson}, an unbiased estimate of the precision matrix $\bP = \bW^{-1}$ of $\by$ will be given by the corrected expression:
\begin{equation}
\label{eq.Winv.unbiased}
\hat\bP = \frac{M - m_{0} -1}{M} \hat\bW^{-1},
\end{equation}
where $\hat\bW = \frac{1}{M} \insum_{j=1}^{M} \by_{j} \by_{j}^{\dag}$ as before.
Thus, to obtain $\bW^{-1}$, the receiver only needs to take $M>m_{0} + 1$ periodic measurements of $\by$ between iteration cycles, and then broadcast the unbiased estimate $\hat\bP$ of $\bW^{-1}$ to the network's users.

%Hence, we will assume that, at each step, $m$ measurements of the received signal are performed ($m$ being finite,  larger than $m_0+1$) so that the receiver can compute $\widehat\bW(n)^{-1}$, a random estimate of $\bW(n)^{-1}$ with no bias and send it back to all transmitters. \mpierre{Is this paragraph needed? It is already said in the text of Section 4.}

Similarly, in the absence of perfect \acl{CSIT}, the users will need to obtain an unbiased estimate of the unilateral gradient matrices $\bV_{k} = \bH_{k}^{\dag} \bW^{-1} \bH_{k}$ from the broadcasted value of $\bW$ and using imperfect measurements of their channel matrices $\bH_{k}$.
However, an added complication here is that the estimated matrix $\hat\bV_{k}$ must be itself Hermitian \textendash\
%so that the discretization \eqref{eq.XLT.discrete} of \eqref{eq.XLT} remain well-defined
otherwise, $\bQ_{k}$ need not be positive-definite and the algorithm might fail to be well-posed.

To accommodate this requirement, an unbiased Hermitian estimate for $\bV_{k}$ may be obtained from a sample $\bH_{k,1},\dotsc,\bH_{k,M}$ ($M>1$) of $\bH_{k}$ which is subject to zero-mean observational errors (assumed independent across users) via the expression: 
\begin{equation}
\label{eq.V.unbiased}
\hat\bV_{k}
	= \frac{1}{2(M-1)}
	\insum_{j=1}^{M-1} \left(
	\bH_{k,j}^{\dag} \hat \bP \bH_{k,j+1} + \bH_{k,j+1}^{\dag} \hat\bP \bH_{k,j}
	\right),
\end{equation}
where $\hat\bP$ is the unbiased estimate \eqref{eq.Winv.unbiased} of $\bW^{-1}$.
Indeed, if the sample measurements $\bH_{k,j}$ are independent realizations of some random variable $\hat\bH_{k}$ with $\ex[\hat\bH_{k}] = \bH_{k}$, we will have:
\begin{flalign*}
\ex[\hat\bV_{k}]
	&= \frac{1}{2(M-1)}
	\insum_{j=1}^{M-1} \ex
	\big[
	\bH_{k,j}^{\dag} \hat \bP \bH_{k,j+1} + \bH_{k,j+1}^{\dag} \hat\bP \bH_{k,j}
	\big]
	\notag\\
	&= \frac{1}{2(M-1)} \insum_{j=1}^{M-1} 2 \ex[\hat\bH_{k}^{\dag}] \ex[\hat \bP] \ex[\hat \bH_{k}]
	= \bH_{k}^{\dag} \bW^{-1} \bH_{k},
\end{flalign*}
where we have used the independence of the samples to decorrelate the expectations in the second equality, and relied on the unbiasedness of $\hat\bP$ and $\hat\bH_{k}$ for the last one.
Thus, with $\ex[\hat\bV_{k}] = \bV_{k}$, our construction of an unbiased estimator for $\bV_{k}$ is complete.
